# Supplementary material for: The Effects of Data Quality on Machine Learning Performance on Tabular Data
Source: arXiv:2207.14529 source file (2025-05-14)
Supplement: Supplementary file 1 [file appendix_clustering_tables.tex]

\clearpage
\subsection{Detailed Result Tables}
\label{subsec:appendix-clustering-result-tables}
\begin{table*}[!hbp]
    \caption{Performance of clustering results for completeness dimension and Bank dataset.}
    \begin{tabular}{l|r|r|r|r|r|r|r|r|r|r|r}
    & \multicolumn{11}{c}{Adjusted Mutual Information Score} \\ 
    Quality & \multicolumn{1}{r|}{1.00} & \multicolumn{1}{r|}{0.90} & \multicolumn{1}{r|}{0.80} & \multicolumn{1}{r|}{0.70} & \multicolumn{1}{r|}{0.60} & \multicolumn{1}{r|}{0.50} & \multicolumn{1}{r|}{0.40} & \multicolumn{1}{r|}{0.30} & \multicolumn{1}{r|}{0.20} & \multicolumn{1}{r|}{0.10} & \multicolumn{1}{r}{0.00}\\
    \hline
    Agglomerative & 0.0684 & 0.0484 & 0.0635 & 0.0655 & 0.0586 & 0.0469 & 0.0170 & 0.0192 & 0.0139 & 0.0111 & 0.0000\\
    Autoencoder & 0.0000 & 0.0016 & 0.0087 & 0.0049 & 0.0036 & 0.0072 & 0.0078 & 0.0032 & 0.0073 & 0.0037 & 0.0000\\
    Gaussian Mixture & 0.0984 & 0.0562 & 0.0284 & 0.0493 & 0.0364 & 0.0243 & 0.0333 & 0.0137 & 0.0163 & 0.0126 & 0.0000\\
    k-Means & 0.0300 & 0.0256 & 0.0225 & 0.0199 & 0.0172 & 0.0152 & 0.0125 & 0.0101 & 0.0073 & 0.0043 & 0.0000\\
    OPTICS & 0.0055 & 0.0086 & 0.0155 & 0.0295 & 0.0358 & 0.0356 & 0.0362 & 0.0353 & 0.0293 & 0.0194 & 0.0000\\
    \end{tabular}
\end{table*}
\begin{table*}[!hbp]
    \caption{Performance of clustering results for consistent representation dimension and Bank dataset.}
    \begin{tabular}{l|r|r|r|r|r|r|r|r|r|r|r}
    & \multicolumn{11}{c}{Adjusted Mutual Information Score} \\ 
    Quality & \multicolumn{1}{r|}{1.00} & \multicolumn{1}{r|}{0.90} & \multicolumn{1}{r|}{0.80} & \multicolumn{1}{r|}{0.70} & \multicolumn{1}{r|}{0.60} & \multicolumn{1}{r|}{0.50} & \multicolumn{1}{r|}{0.40} & \multicolumn{1}{r|}{0.30} & \multicolumn{1}{r|}{0.27} & \multicolumn{1}{r|}{0.24} & \multicolumn{1}{r}{0.21}\\
    \hline
    Agglomerative & 0.1153 & 0.0381 & 0.0071 & 0.0113 & 0.0117 & 0.0150 & 0.0034 & 0.0115 & 0.0213 & 0.0204 & 0.0210\\
    Autoencoder & 0.0000 & 0.0060 & 0.0058 & 0.0242 & 0.0182 & 0.0248 & 0.0243 & 0.0200 & 0.0187 & 0.0122 & 0.0122\\
    Gaussian Mixture & 0.0707 & 0.0588 & 0.0522 & 0.0419 & 0.0459 & 0.0571 & 0.0360 & 0.0379 & 0.0430 & 0.0513 & 0.0550\\
    k-Means & 0.0300 & 0.0301 & 0.0304 & 0.0307 & 0.0298 & 0.0303 & 0.0297 & 0.0301 & 0.0301 & 0.0300 & 0.0300\\
    OPTICS & 0.0040 & 0.0049 & 0.0050 & 0.0048 & 0.0068 & 0.0058 & 0.0050 & 0.0043 & 0.0061 & 0.0053 & 0.0054\\
    \end{tabular}
\end{table*}

\begin{table*}[!hbp]
    \caption{Performance of clustering results for feature accuracy dimension and Bank dataset.}
    \begin{tabular}{l|r|r|r|r|r|r|r|r|r|r|r}
    & \multicolumn{11}{c}{Adjusted Mutual Information Score} \\ 
    Quality & \multicolumn{1}{r|}{1.00} & \multicolumn{1}{r|}{0.91} & \multicolumn{1}{r|}{0.81} & \multicolumn{1}{r|}{0.72} & \multicolumn{1}{r|}{0.63} & \multicolumn{1}{r|}{0.53} & \multicolumn{1}{r|}{0.44} & \multicolumn{1}{r|}{0.35} & \multicolumn{1}{r|}{0.25} & \multicolumn{1}{r|}{0.16} & \multicolumn{1}{r}{0.07}\\
    \hline
    Agglomerative & 0.0684 & 0.0474 & 0.0414 & 0.0160 & 0.0196 & 0.0114 & 0.0114 & 0.0039 & 0.0016 & 0.0002 & 0.0029\\
    Autoencoder & 0.0000 & 0.0000 & 0.0327 & 0.0110 & 0.0076 & 0.0124 & 0.0038 & 0.0031 & 0.0024 & 0.0015 & 0.0015\\
    Gaussian Mixture & 0.0984 & 0.0729 & 0.0691 & 0.0358 & 0.0393 & 0.0291 & 0.0256 & 0.0099 & 0.0025 & 0.0000 & 0.0019\\
    k-Means & 0.0300 & 0.0244 & 0.0172 & 0.0110 & 0.0075 & 0.0058 & 0.0039 & 0.0027 & 0.0027 & 0.0019 & 0.0018\\
    OPTICS & 0.0055 & 0.0873 & 0.0645 & 0.0493 & 0.0344 & 0.0176 & 0.0066 & 0.0001 & 0.0000 & 0.0002 & 0.0001\\
    \end{tabular}
\end{table*}

\begin{table*}[!hbp]
    \caption{Performance of clustering results for target accuracy dimension and Bank dataset.}
    \begin{tabular}{l|r|r|r|r|r|r|r|r|r|r|r}
    & \multicolumn{11}{c}{Adjusted Mutual Information Score} \\ 
    Quality & \multicolumn{1}{r|}{1.00} & \multicolumn{1}{r|}{0.90} & \multicolumn{1}{r|}{0.80} & \multicolumn{1}{r|}{0.70} & \multicolumn{1}{r|}{0.60} & \multicolumn{1}{r|}{0.50} & \multicolumn{1}{r|}{0.40} & \multicolumn{1}{r|}{0.30} & \multicolumn{1}{r|}{0.20} & \multicolumn{1}{r|}{0.10} & \multicolumn{1}{r}{0.00}\\
    \hline
    Agglomerative & 0.0684 & 0.0528 & 0.0384 & 0.0275 & 0.0180 & 0.0119 & 0.0062 & 0.0016 & 0.0001 & 0.0007 & 0.0042\\
    Autoencoder & 0.0000 & 0.0000 & 0.0000 & 0.0000 & 0.0000 & 0.0000 & 0.0000 & 0.0000 & 0.0000 & 0.0000 & 0.0000\\
    Gaussian Mixture & 0.0984 & 0.0759 & 0.0545 & 0.0378 & 0.0262 & 0.0161 & 0.0076 & 0.0018 & 0.0001 & 0.0005 & 0.0045\\
    k-Means & 0.0300 & 0.0227 & 0.0171 & 0.0122 & 0.0078 & 0.0052 & 0.0020 & 0.0006 & 0.0001 & 0.0001 & 0.0015\\
    OPTICS & 0.0055 & 0.0047 & 0.0033 & 0.0024 & 0.0017 & 0.0013 & 0.0007 & 0.0002 & 0.0001 & 0.0001 & 0.0004\\
    \end{tabular}
\end{table*}

\begin{table*}[!hbp]
    \caption{Performance of clustering results for target class balance dimension and Bank dataset.}
    \begin{tabular}{l|r|r|r|r|r|r|r|r|r|r|r}
    & \multicolumn{11}{c}{Adjusted Mutual Information Score} \\ 
    Quality & \multicolumn{1}{r|}{1.00} & \multicolumn{1}{r|}{0.86} & \multicolumn{1}{r|}{0.74} & \multicolumn{1}{r|}{0.64} & \multicolumn{1}{r|}{0.56} & \multicolumn{1}{r|}{0.48} & \multicolumn{1}{r|}{0.42} & \multicolumn{1}{r|}{0.36} & \multicolumn{1}{r|}{0.31} & \multicolumn{1}{r|}{0.26} & \multicolumn{1}{r}{0.23}\\
    \hline
    Agglomerative & 0.1153 & 0.1131 & 0.0886 & 0.1115 & 0.0676 & 0.1234 & 0.1011 & 0.0866 & 0.0632 & 0.0842 & 0.1087\\
    Autoencoder & 0.0000 & 0.0000 & 0.0000 & 0.0000 & 0.0000 & 0.0000 & 0.0000 & 0.0000 & 0.0000 & 0.0000 & 0.0000\\
    Gaussian Mixture & 0.0707 & 0.0786 & 0.0923 & 0.0894 & 0.0857 & 0.0726 & 0.0934 & 0.0977 & 0.0687 & 0.1118 & 0.1033\\
    k-Means & 0.0300 & 0.0282 & 0.0275 & 0.0263 & 0.0251 & 0.0236 & 0.0223 & 0.0210 & 0.0196 & 0.0174 & 0.0166\\
    OPTICS & 0.0040 & 0.0045 & 0.0045 & 0.0033 & 0.0046 & 0.0042 & 0.0045 & 0.0048 & 0.0051 & 0.0036 & 0.0030\\
    \end{tabular}
\end{table*}

\begin{table*}[!hbp]
    \caption{Performance of clustering results for uniqueness dimension and Bank dataset.}
    \begin{tabular}{l|r|r|r|r|r|r|r|r|r}
    & \multicolumn{9}{c}{Adjusted Mutual Information Score} \\ 
    Quality & \multicolumn{1}{r|}{1.00} & \multicolumn{1}{r|}{0.90} & \multicolumn{1}{r|}{0.80} & \multicolumn{1}{r|}{0.70} & \multicolumn{1}{r|}{0.60} & \multicolumn{1}{r|}{0.50} & \multicolumn{1}{r|}{0.40} & \multicolumn{1}{r|}{0.30} & \multicolumn{1}{r}{0.20}\\
    \hline
    Agglomerative & 0.0366 & 0.0467 & 0.0371 & 0.0365 & 0.0455 & 0.0482 & 0.0505 & 0.0369 & 0.0505\\
    Autoencoder & 0.0000 & 0.0000 & 0.0000 & 0.0000 & 0.0000 & 0.0000 & 0.0000 & 0.0000 & 0.0000\\
    Gaussian Mixture & 0.0194 & 0.0155 & 0.0227 & 0.0332 & 0.0275 & 0.0311 & 0.0298 & 0.0332 & 0.0311\\
    k-Means & 0.0147 & 0.0156 & 0.0188 & 0.0210 & 0.0227 & 0.0212 & 0.0245 & 0.0274 & 0.0225\\
    OPTICS & 0.0118 & 0.0101 & 0.0065 & 0.0082 & 0.0077 & 0.0073 & 0.0098 & 0.0092 & 0.0067\\
    \end{tabular}
\end{table*}

\begin{table*}[!hbp]
    \caption{Performance of clustering results for completeness dimension and Covertype dataset.}
    \begin{tabular}{l|r|r|r|r|r|r|r|r|r|r|r}
    & \multicolumn{11}{c}{Adjusted Mutual Information Score} \\ 
    Quality & \multicolumn{1}{r|}{1.00} & \multicolumn{1}{r|}{0.90} & \multicolumn{1}{r|}{0.80} & \multicolumn{1}{r|}{0.70} & \multicolumn{1}{r|}{0.60} & \multicolumn{1}{r|}{0.50} & \multicolumn{1}{r|}{0.40} & \multicolumn{1}{r|}{0.30} & \multicolumn{1}{r|}{0.20} & \multicolumn{1}{r|}{0.10} & \multicolumn{1}{r}{0.00}\\
    \hline
    Agglomerative & 0.3524 & 0.0002 & 0.0005 & 0.0032 & 0.0036 & 0.0135 & 0.0036 & 0.0005 & 0.0002 & 0.0000 & 0.0000\\
    Autoencoder & 0.1222 & 0.1441 & 0.1073 & 0.0617 & 0.0486 & 0.0403 & 0.0360 & 0.0242 & 0.0094 & 0.0196 & 0.0000\\
    Gaussian Mixture & 0.3540 & 0.2421 & 0.2169 & 0.1716 & 0.1255 & 0.1055 & 0.0726 & 0.0530 & 0.0328 & 0.0094 & 0.0000\\
    k-Prototypes & 0.1937 & 0.1389 & 0.0996 & 0.0625 & 0.0529 & 0.0437 & 0.0353 & 0.0278 & 0.0188 & 0.0104\\
    OPTICS & 0.0244 & 0.0024 & 0.0065 & 0.0046 & 0.0014 & 0.0001 & 0.0002 & 0.0030 & 0.0072 & 0.0116 & 0.0000\\
    \end{tabular}
\end{table*}

\begin{table*}[!hbp]
    \caption{Performance of clustering results for consistent representation dimension and Covertype dataset.}
    \begin{tabular}{l|r|r|r|r|r|r|r|r|r|r|r}
    & \multicolumn{11}{c}{Adjusted Mutual Information Score} \\ 
    Quality & \multicolumn{1}{r|}{1.00} & \multicolumn{1}{r|}{0.90} & \multicolumn{1}{r|}{0.80} & \multicolumn{1}{r|}{0.70} & \multicolumn{1}{r|}{0.60} & \multicolumn{1}{r|}{0.50} & \multicolumn{1}{r|}{0.40} & \multicolumn{1}{r|}{0.30} & \multicolumn{1}{r|}{0.26} & \multicolumn{1}{r|}{0.23} & \multicolumn{1}{r}{0.21}\\
    \hline
    Agglomerative & 0.3524 & 0.0768 & 0.0000 & 0.0000 & 0.0000 & 0.0001 & 0.0002 & 0.0009 & 0.0006 & 0.0007 & 0.0007\\
    Autoencoder & 0.1378 & 0.1115 & 0.1365 & 0.1234 & 0.0417 & 0.0401 & 0.1064 & 0.0709 & 0.0363 & 0.1176 & 0.1168\\
    Gaussian Mixture & 0.3277 & 0.3051 & 0.2794 & 0.2892 & 0.2901 & 0.2962 & 0.3049 & 0.3059 & 0.3066 & 0.3045 & 0.3014\\
    k-Prototypes & 0.1939 & 0.1937 & 0.1937 & 0.1938 & 0.1937 & 0.1938 & 0.1938 & 0.1938 & 0.1938 & 0.1938 & 0.1938\\
    OPTICS & 0.0244 & 0.0190 & 0.0244 & 0.0190 & 0.0190 & 0.0190 & 0.0190 & 0.0190 & 0.0244 & 0.0190 & 0.0244\\
    \end{tabular}
\end{table*}

\begin{table*}[!hbp]
    \caption{Performance of clustering results for feature accuracy dimension and Covertype dataset.}
    \begin{tabular}{l|r|r|r|r|r|r|r|r|r|r|r}
    & \multicolumn{11}{c}{Adjusted Mutual Information Score} \\ 
    Quality & \multicolumn{1}{r|}{1.00} & \multicolumn{1}{r|}{0.91} & \multicolumn{1}{r|}{0.82} & \multicolumn{1}{r|}{0.73} & \multicolumn{1}{r|}{0.64} & \multicolumn{1}{r|}{0.56} & \multicolumn{1}{r|}{0.47} & \multicolumn{1}{r|}{0.38} & \multicolumn{1}{r|}{0.29} & \multicolumn{1}{r|}{0.20} & \multicolumn{1}{r}{0.11}\\
    \hline
    Agglomerative & 0.3524 & 0.0000 & 0.0001 & 0.0009 & 0.0005 & 0.0001 & 0.0007 & 0.0010 & 0.0002 & 0.0001 & 0.3324\\
    Autoencoder & 0.1222 & 0.1144 & 0.0700 & 0.0819 & 0.0668 & 0.0579 & 0.0438 & 0.0487 & 0.0342 & 0.0223 & 0.0239\\
    Gaussian Mixture & 0.3540 & 0.0438 & 0.0264 & 0.0232 & 0.0724 & 0.0514 & 0.0396 & 0.0069 & 0.0025 & 0.0229 & 0.2805\\
    k-Prototypes & 0.1937 & 0.1856 & 0.1680 & 0.1323 & 0.1103 & 0.0910 & 0.0736 & 0.0626 & 0.0519 & 0.0441 & 0.0396\\
    OPTICS & 0.0244 & 0.0000 & 0.0000 & 0.0000 & 0.0003 & 0.0000 & 0.0006 & 0.0000 & 0.0000 & 0.0004 & 0.0000\\
    \end{tabular}
\end{table*}

\begin{table*}[!hbp]
    \caption{Performance of clustering results for target accuracy dimension and Covertype dataset.}
    \begin{tabular}{l|r|r|r|r|r|r|r|r|r|r|r}
    & \multicolumn{11}{c}{Adjusted Mutual Information Score} \\ 
    Quality & \multicolumn{1}{r|}{1.00} & \multicolumn{1}{r|}{0.90} & \multicolumn{1}{r|}{0.80} & \multicolumn{1}{r|}{0.70} & \multicolumn{1}{r|}{0.60} & \multicolumn{1}{r|}{0.50} & \multicolumn{1}{r|}{0.40} & \multicolumn{1}{r|}{0.30} & \multicolumn{1}{r|}{0.20} & \multicolumn{1}{r|}{0.10} & \multicolumn{1}{r}{0.00}\\
    \hline
    Agglomerative & 0.3524 & 0.2475 & 0.1790 & 0.1225 & 0.0840 & 0.0501 & 0.0264 & 0.0111 & 0.0013 & 0.0009 & 0.0102\\
    Autoencoder & 0.1222 & 0.0886 & 0.0640 & 0.0440 & 0.0296 & 0.0179 & 0.0099 & 0.0037 & 0.0004 & 0.0004 & 0.0028\\
    Gaussian Mixture & 0.3540 & 0.2534 & 0.1831 & 0.1283 & 0.0862 & 0.0526 & 0.0269 & 0.0108 & 0.0013 & 0.0007 & 0.0100\\
    k-Prototypes & 0.1937 & 0.1421 & 0.1019 & 0.0703 & 0.0477 & 0.0283 & 0.0150 & 0.0054 & 0.0006 & 0.0005 & 0.0043\\
    OPTICS & 0.0244 & 0.0186 & 0.0148 & 0.0107 & 0.0071 & 0.0047 & 0.0028 & 0.0011 & 0.0000 & 0.0001 & 0.0019\\
    \end{tabular}
\end{table*}

\begin{table*}[!hbp]
    \caption{Performance of clustering results for target class balance dimension and Covertype dataset.}
    \begin{tabular}{l|r|r|r|r|r|r|r|r|r|r|r}
    & \multicolumn{11}{c}{Adjusted Mutual Information Score} \\ 
    Quality & \multicolumn{1}{r|}{1.00} & \multicolumn{1}{r|}{0.86} & \multicolumn{1}{r|}{0.74} & \multicolumn{1}{r|}{0.64} & \multicolumn{1}{r|}{0.56} & \multicolumn{1}{r|}{0.48} & \multicolumn{1}{r|}{0.42} & \multicolumn{1}{r|}{0.36} & \multicolumn{1}{r|}{0.31} & \multicolumn{1}{r|}{0.26} & \multicolumn{1}{r}{0.23}\\
    \hline
    Agglomerative & 0.3524 & 0.3320 & 0.3245 & 0.3218 & 0.3111 & 0.3033 & 0.2953 & 0.2922 & 0.2832 & 0.2750 & 0.2688\\
    Autoencoder & 0.1378 & 0.0403 & 0.0950 & 0.1562 & 0.1487 & 0.1537 & 0.1455 & 0.1730 & 0.1349 & 0.1343 & 0.1327\\
    Gaussian Mixture & 0.3277 & 0.3150 & 0.2959 & 0.3104 & 0.3178 & 0.3152 & 0.2925 & 0.3033 & 0.3122 & 0.3019 & 0.2891\\
    k-Prototypes & 0.1939 & 0.1905 & 0.1874 & 0.1846 & 0.1825 & 0.1799 & 0.1771 & 0.1750 & 0.1738 & 0.1699 & 0.1674\\
    OPTICS & 0.0244 & 0.0227 & 0.0138 & 0.0322 & 0.0116 & 0.0014 & 0.0003 & 0.0012 & 0.0006 & 0.0005 & 0.0054\\
    \end{tabular}
\end{table*}

\begin{table*}[!hbp]
    \caption{Performance of clustering results for uniqueness dimension and Covertype dataset.}
    \begin{tabular}{l|r|r|r|r|r|r|r|r|r}
    & \multicolumn{9}{c}{Adjusted Mutual Information Score} \\ 
    Quality & \multicolumn{1}{r|}{1.00} & \multicolumn{1}{r|}{0.90} & \multicolumn{1}{r|}{0.80} & \multicolumn{1}{r|}{0.70} & \multicolumn{1}{r|}{0.60} & \multicolumn{1}{r|}{0.50} & \multicolumn{1}{r|}{0.40} & \multicolumn{1}{r|}{0.30} & \multicolumn{1}{r}{0.20}\\
    \hline
    Agglomerative & 0.3524 & 0.3388 & 0.3390 & 0.3321 & 0.3450 & 0.3487 & 0.3401 & 0.3338 & 0.3405\\
    Autoencoder & 0.1222 & 0.1210 & 0.0820 & 0.1530 & 0.0993 & 0.0851 & 0.0734 & 0.0766 & 0.0748\\
    Gaussian Mixture & 0.3540 & 0.3226 & 0.3206 & 0.3310 & 0.3248 & 0.3403 & 0.3304 & 0.3224 & 0.3205\\
    k-Prototypes & 0.1937 & 0.1944 & 0.1927 & 0.1941 & 0.1932 & 0.1984 & 0.1975 & 0.1970 & 0.1982\\
    OPTICS & 0.0244 & 0.0257 & 0.0508 & 0.0418 & 0.0744 & 0.1073 & 0.1355 & 0.1821 & 0.2092\\
    \end{tabular}
\end{table*}

\begin{table*}[!hbp]
    \caption{Performance of clustering results for completeness dimension and Letter dataset.}
    \begin{tabular}{l|r|r|r|r|r|r|r|r|r|r|r}
    & \multicolumn{11}{c}{Adjusted Mutual Information Score} \\ 
    Quality & \multicolumn{1}{r|}{1.00} & \multicolumn{1}{r|}{0.90} & \multicolumn{1}{r|}{0.80} & \multicolumn{1}{r|}{0.70} & \multicolumn{1}{r|}{0.60} & \multicolumn{1}{r|}{0.50} & \multicolumn{1}{r|}{0.40} & \multicolumn{1}{r|}{0.30} & \multicolumn{1}{r|}{0.20} & \multicolumn{1}{r|}{0.10} & \multicolumn{1}{r}{0.00}\\
    \hline
    Agglomerative & 0.4019 & 0.1208 & 0.0451 & 0.0246 & 0.0145 & 0.0101 & 0.0065 & 0.0050 & 0.0021 & 0.0023 & 0.0000\\
    Autoencoder & 0.0655 & 0.0635 & 0.0289 & 0.0299 & 0.0205 & 0.0376 & 0.0098 & 0.0176 & 0.0095 & 0.0239 & 0.0000\\
    Gaussian Mixture & 0.4437 & 0.1181 & 0.0402 & 0.0075 & 0.0021 & 0.0008 & 0.0009 & 0.0012 & 0.0009 & 0.0007 & 0.0000\\
    k-Means & 0.3515 & 0.1352 & 0.0600 & 0.0325 & 0.0206 & 0.0122 & 0.0140 & 0.0144 & 0.0136 & 0.0122 & 0.0000\\
    OPTICS & 0.1882 & 0.0000 & 0.0000 & 0.0000 & 0.0000 & 0.0000 & 0.0000 & 0.0003 & 0.0005 & 0.0000 & 0.0000\\
    \end{tabular}
\end{table*}

\begin{table*}[!hbp]
    \caption{Performance of clustering results for feature accuracy dimension and Letter dataset.}
    \begin{tabular}{l|r|r|r|r|r|r|r|r|r|r|r}
    & \multicolumn{11}{c}{Adjusted Mutual Information Score} \\ 
    Quality & \multicolumn{1}{r|}{1.00} & \multicolumn{1}{r|}{0.92} & \multicolumn{1}{r|}{0.84} & \multicolumn{1}{r|}{0.76} & \multicolumn{1}{r|}{0.68} & \multicolumn{1}{r|}{0.60} & \multicolumn{1}{r|}{0.52} & \multicolumn{1}{r|}{0.44} & \multicolumn{1}{r|}{0.36} & \multicolumn{1}{r|}{0.28} & \multicolumn{1}{r}{0.20}\\
    \hline
    Agglomerative & 0.4019 & 0.3797 & 0.3059 & 0.2107 & 0.1331 & 0.0824 & 0.0541 & 0.0366 & 0.0262 & 0.0195 & 0.0158\\
    Autoencoder & 0.0655 & 0.0607 & 0.0538 & 0.0661 & 0.0234 & 0.0314 & 0.0224 & 0.0134 & 0.0123 & 0.0091 & 0.0087\\
    Gaussian Mixture & 0.4437 & 0.4647 & 0.3732 & 0.2704 & 0.1818 & 0.1095 & 0.0691 & 0.0442 & 0.0299 & 0.0227 & 0.0167\\
    k-Means & 0.3515 & 0.3406 & 0.3047 & 0.2378 & 0.1651 & 0.1079 & 0.0739 & 0.0501 & 0.0324 & 0.0260 & 0.0192\\
    OPTICS & 0.1882 & 0.0000 & 0.0000 & 0.0000 & 0.0000 & 0.0000 & 0.0000 & 0.0000 & 0.0000 & 0.0000 & 0.0000\\
    \end{tabular}
\end{table*}

\begin{table*}[!hbp]
    \caption{Performance of clustering results for target accuracy dimension and Letter dataset.}
    \begin{tabular}{l|r|r|r|r|r|r|r|r|r|r|r}
    & \multicolumn{11}{c}{Adjusted Mutual Information Score} \\ 
    Quality & \multicolumn{1}{r|}{1.00} & \multicolumn{1}{r|}{0.90} & \multicolumn{1}{r|}{0.80} & \multicolumn{1}{r|}{0.70} & \multicolumn{1}{r|}{0.60} & \multicolumn{1}{r|}{0.50} & \multicolumn{1}{r|}{0.40} & \multicolumn{1}{r|}{0.30} & \multicolumn{1}{r|}{0.20} & \multicolumn{1}{r|}{0.10} & \multicolumn{1}{r}{0.00}\\
    \hline
    Agglomerative & 0.4019 & 0.3176 & 0.2501 & 0.1909 & 0.1416 & 0.0992 & 0.0660 & 0.0361 & 0.0153 & 0.0025 & 0.0016\\
    Autoencoder & 0.0655 & 0.0522 & 0.0402 & 0.0304 & 0.0229 & 0.0156 & 0.0105 & 0.0057 & 0.0020 & 0.0006 & 0.0001\\
    Gaussian Mixture & 0.4437 & 0.3530 & 0.2767 & 0.2148 & 0.1602 & 0.1134 & 0.0754 & 0.0429 & 0.0190 & 0.0034 & 0.0021\\
    k-Means & 0.3515 & 0.2785 & 0.2179 & 0.1651 & 0.1238 & 0.0873 & 0.0565 & 0.0318 & 0.0132 & 0.0027 & 0.0007\\
    OPTICS & 0.1882 & 0.1527 & 0.1219 & 0.0936 & 0.0702 & 0.0511 & 0.0328 & 0.0182 & 0.0084 & 0.0013 & 0.0013\\
    \end{tabular}
\end{table*}

\begin{table*}[!hbp]
    \caption{Performance of clustering results for target class balance dimension and Letter dataset.}
    \begin{tabular}{l|r|r|r|r|r|r|r|r|r|r|r}
    & \multicolumn{11}{c}{Adjusted Mutual Information Score} \\ 
    Quality & \multicolumn{1}{r|}{1.00} & \multicolumn{1}{r|}{0.89} & \multicolumn{1}{r|}{0.80} & \multicolumn{1}{r|}{0.71} & \multicolumn{1}{r|}{0.61} & \multicolumn{1}{r|}{0.56} & \multicolumn{1}{r|}{0.50} & \multicolumn{1}{r|}{0.43} & \multicolumn{1}{r|}{0.39} & \multicolumn{1}{r|}{0.36} & \multicolumn{1}{r}{0.32}\\
    \hline
    Agglomerative & 0.4019 & 0.4010 & 0.4000 & 0.4047 & 0.4110 & 0.4100 & 0.4104 & 0.4065 & 0.4190 & 0.4205 & 0.4193\\
    Autoencoder & 0.0655 & 0.0508 & 0.0738 & 0.0494 & 0.0963 & 0.0826 & 0.0550 & 0.1353 & 0.1418 & 0.0716 & 0.1278\\
    Gaussian Mixture & 0.4437 & 0.4426 & 0.4434 & 0.4417 & 0.4603 & 0.4590 & 0.4542 & 0.4637 & 0.4691 & 0.4723 & 0.4755\\
    k-Means & 0.3515 & 0.3509 & 0.3544 & 0.3556 & 0.3548 & 0.3602 & 0.3593 & 0.3670 & 0.3675 & 0.3698 & 0.3767\\
    OPTICS & 0.1882 & 0.2016 & 0.1988 & 0.2117 & 0.2191 & 0.2127 & 0.2204 & 0.2210 & 0.2221 & 0.2276 & 0.2356\\
    \end{tabular}
\end{table*}

\begin{table*}[!hbp]
    \caption{Performance of clustering results for uniqueness dimension and Letter dataset.}
    \begin{tabular}{l|r|r|r|r|r|r|r|r|r}
    & \multicolumn{9}{c}{Adjusted Mutual Information Score} \\ 
    Quality & \multicolumn{1}{r|}{1.00} & \multicolumn{1}{r|}{0.90} & \multicolumn{1}{r|}{0.80} & \multicolumn{1}{r|}{0.70} & \multicolumn{1}{r|}{0.60} & \multicolumn{1}{r|}{0.50} & \multicolumn{1}{r|}{0.40} & \multicolumn{1}{r|}{0.30} & \multicolumn{1}{r}{0.20}\\
    \hline
    Agglomerative & 0.3995 & 0.3934 & 0.4020 & 0.4004 & 0.4071 & 0.4082 & 0.4062 & 0.4047 & 0.4050\\
    Autoencoder & 0.0904 & 0.1166 & 0.1047 & 0.0959 & 0.0948 & 0.0841 & 0.0822 & 0.1371 & 0.1932\\
    Gaussian Mixture & 0.4277 & 0.4380 & 0.4409 & 0.4229 & 0.4385 & 0.4300 & 0.4304 & 0.4290 & 0.4380\\
    k-Means & 0.3519 & 0.3530 & 0.3603 & 0.3552 & 0.3632 & 0.3653 & 0.3694 & 0.3700 & 0.3703\\
    OPTICS & 0.1882 & 0.2034 & 0.2129 & 0.2139 & 0.2629 & 0.3128 & 0.3387 & 0.3418 & 0.3502\\
    \end{tabular}
\end{table*}
